# Supplementary material for: The Stochastic Topic Block Model for the Clustering of Vertices in Networks with Textual Edges
Source: arXiv:1610.02427 ancillary file (2017-01-16)
Supplement: Supplementary file 1 [file STBM-supp.pdf]

Noname manuscript No.
(will be inserted by the editor)

# Supplementary Material for "The Stochastic Topic Block Model for the Clustering of Vertices in Networks with Textual Edges"


C. Bouveyron · P. Latouche · R. Zreik



Received: date / Accepted: date


## 1 Analysis of the Enron email network

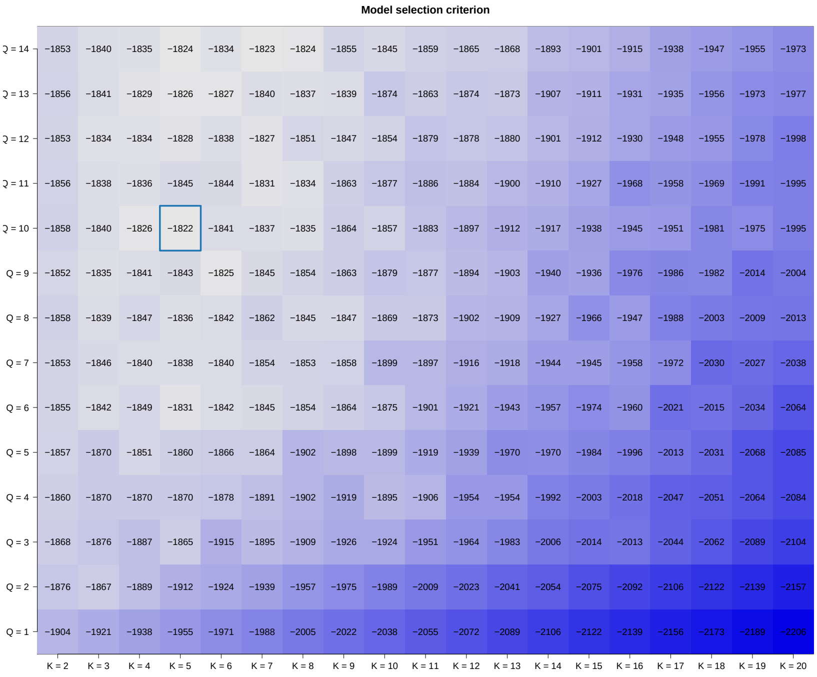


**Fig. 1** Model selection for STBM on the Enron data set. The values of ICL are divided by $10^3$.


Address(es) of author(s) should be given

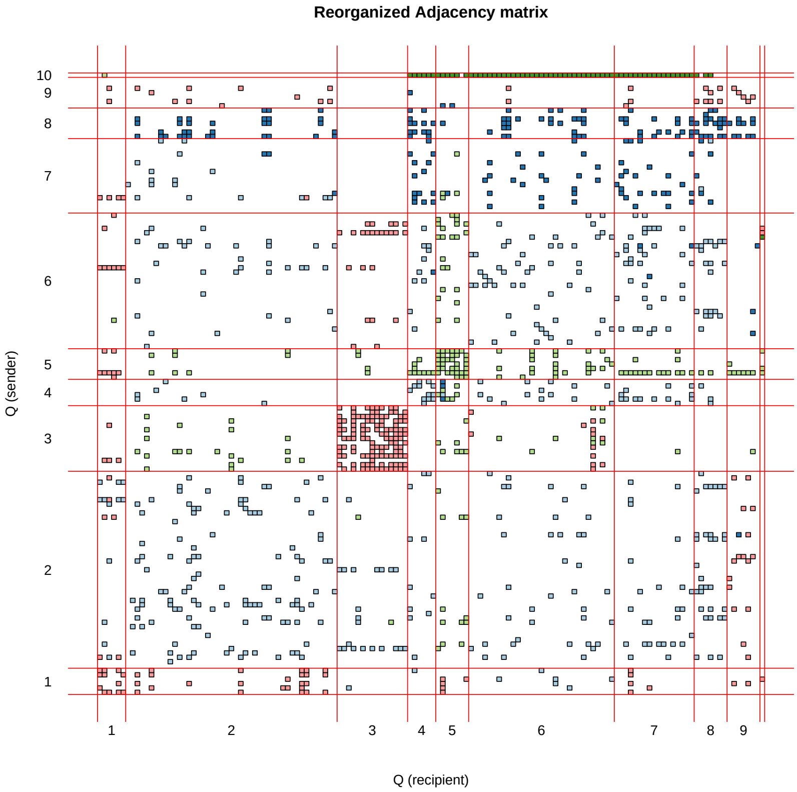


**Fig. 2** Reorganized adjacency matrix according to groups for STBM on the Enron data set.

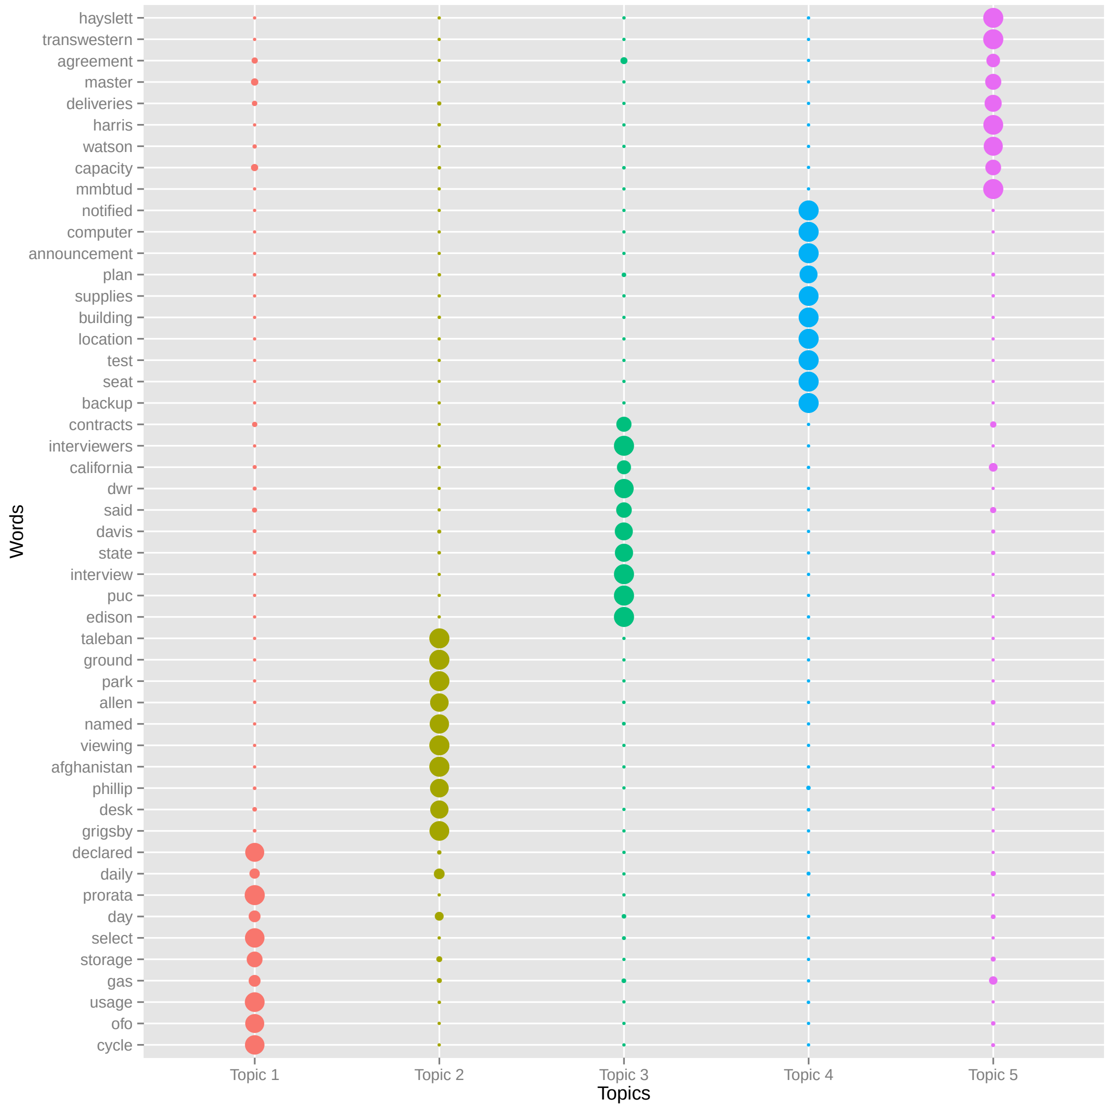


**Fig. 3** Specificity of a selection of words regarding the 5 found topics by STBM on the Enron data set.

## 2 Analysis of the Nips'15 co-authorship network

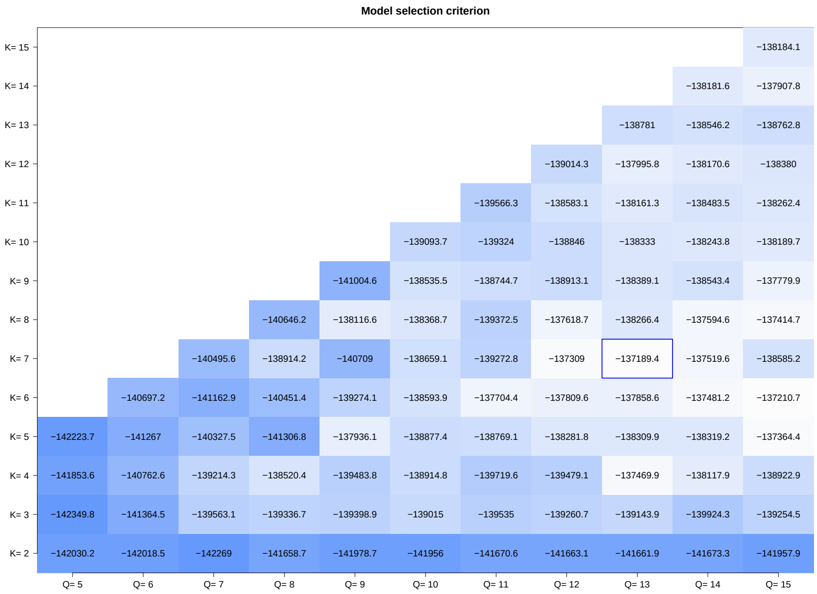


**Fig. 4** Model selection for STBM on the NIPS co-authorship network. The values of ICL are divided by $10^3$.

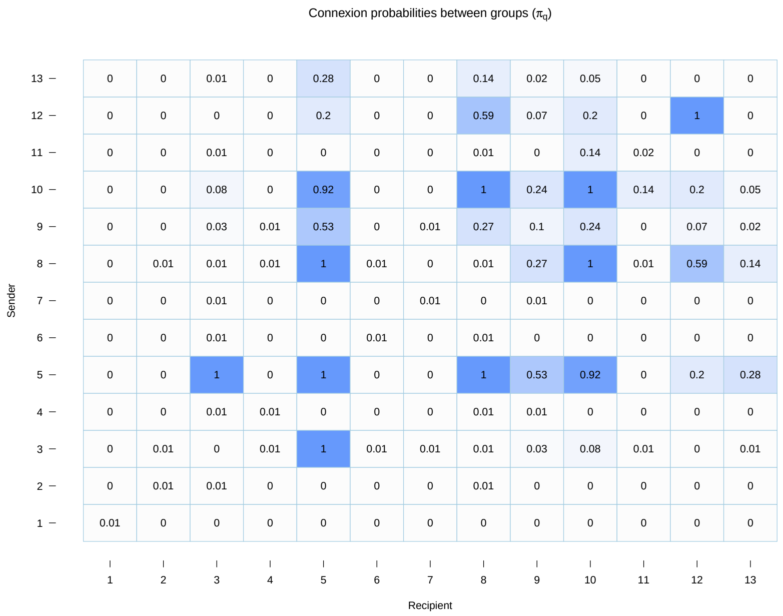


**Fig. 5** Estimated matrix $\pi$ by STBM on the Nips co-authorship network.

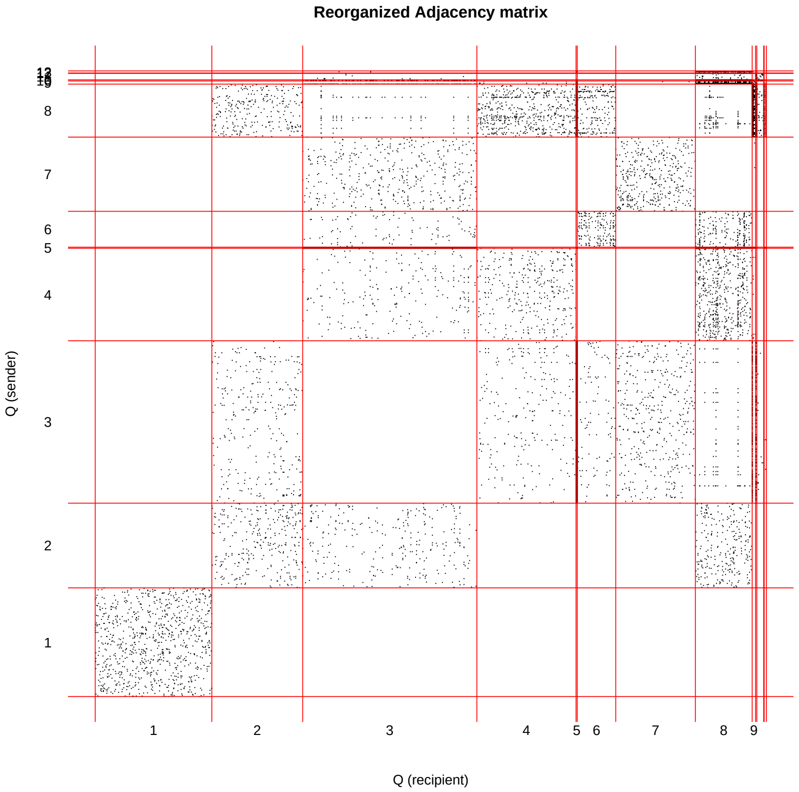


**Fig. 6** Reorganized adjacency matrix according to groups for STBM on the Nips co-authorship network.

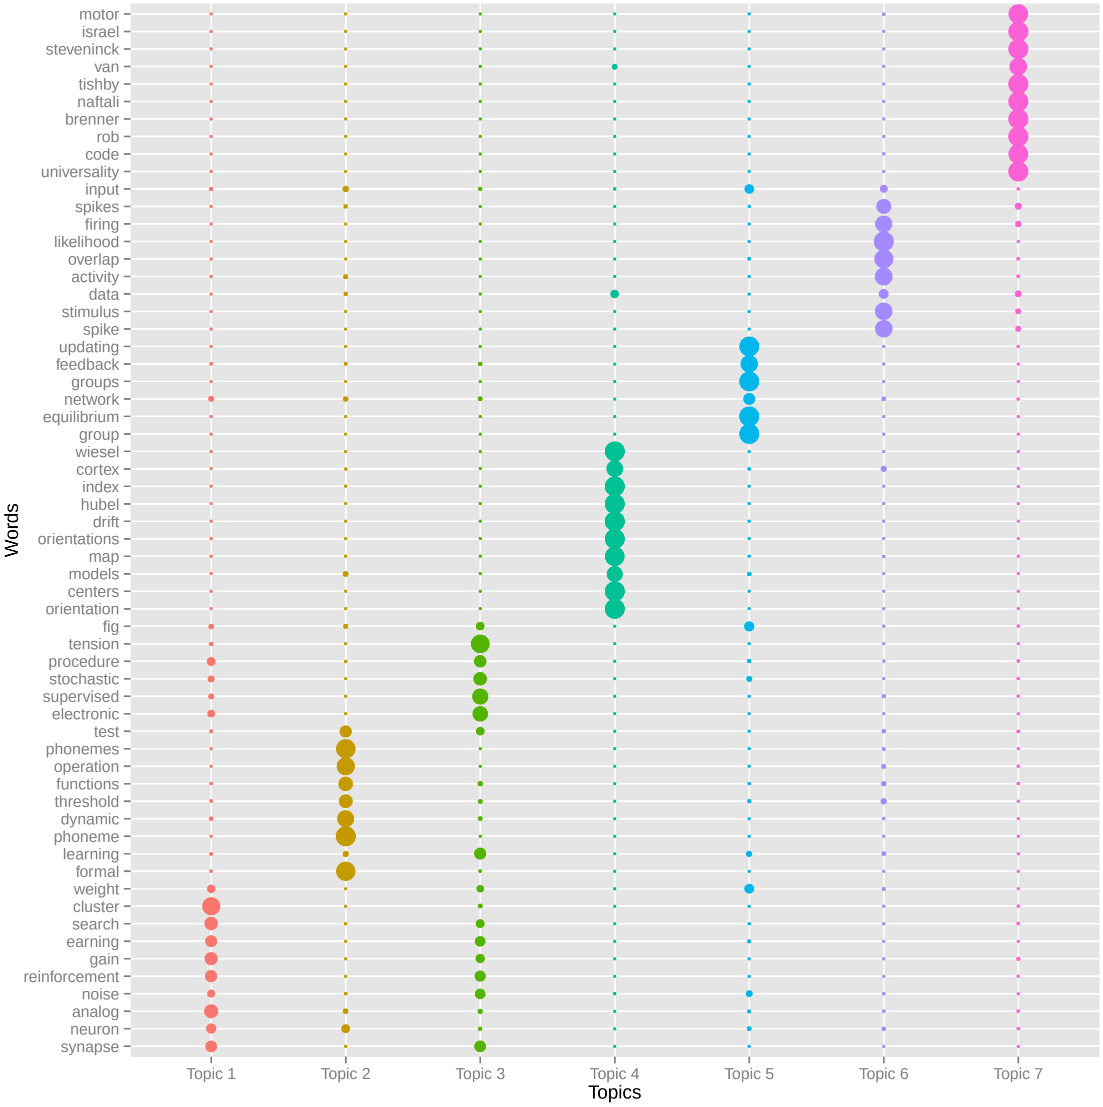


**Fig. 7** Specificity of a selection of words regarding the 5 found topics by STBM on the Nips co-authorship network.
